# Supplementary material for: Cavity-Enhanced Photon Emission from a Single Germanium-Vacancy Center in a Diamond Membrane
Source: arXiv:1912.05247 ancillary file (2020-05-25)
Supplement: Supplementary file 1 [file Supplement.pdf]

# Supplemental Material: Cavity-Enhanced Photon Emission from a Single Germanium Vacancy Center in a Diamond Membrane

Rasmus Høy Jensen,[1,*] Erika Janitz,[2,*] Yannik Fontana,[1] Yi He,[3] Olivier Gobron,[1] Ilya P. Radko,[1] Mihir Bhaskar,[4] Ruffin Evans,[4] César Daniel Rodríguez Rosenblueth,[2] Lilian Childress,[2] Alexander Huck,[1] and Ulrik Lund Andersen[1]

[1]*Center for Macroscopic Quantum States (bigQ), Department of Physics, Technical University of Denmark, Lyngby, Denmark*
[2]*Department of Physics, McGill University, Montreal, Quebec, Canada*
[3]*Department of Electrical and Computer Engineering, Carnegie Mellon University, Pittsburgh, Pennsylvania 15213, USA*
[4]*Department of Physics, Harvard University, Cambridge, Massachusetts 02138, USA*

## I. DIAMOND MEMBRANE FABRICATION

The diamond membrane sample was fabricated from a ⟨100⟩-cut electronic-grade bulk diamond (Element 6), which was laser-cut laterally into $20 \pm 10$ µm thick diamond plates (Delaware Diamond Knives). We cleaned one of the resulting membranes in a 2:1 piranha solution before bonding it (via Van der Waals forces) to a sapphire carrier wafer. We then employed a cycled $ArCl_2$ and $O_2/Ar$ dry-etching process [50–52] to remove 4 µm of material, thereby smoothing the surface and relieving material strain from polishing. The etched surface was then implanted with germanium ions at an energy of 330 keV and fluence of $10^9/\mathrm{cm}^2$, corresponding to an approximate implantation depth of $h = \lambda/(2n_d) \approx 125 \pm 20$ nm (calculated using SRIM software [53]). The membrane was then cleaned in a triacid solution (1:1:1 sulfuric, nitric, and perchloric acids) and annealed using a three step procedure [54]. After annealing, we again cleaned the sample with a triacid mixture to remove graphitization and bonded it (implanted side down) to a carrier wafer for further etching to the desired device thickness (≈1 µm). The membrane was then removed from the carrier in a boiling piranha solution, rinsed in deionized water, and transferred in a water droplet (implanted side down) onto the flat mirror, where it was blow-dried with nitrogen. Confocal characterization of these samples showed ≈ 6% annealing conversion efficiency from implanted ions to GeV centers.

## II. SINGLE PHOTON EMISSION

We ensure that we are studying a single GeV center by measuring the second order correlation function (as seen in Fig. 1 for $P = 19$ mW pump power) and fitting Eq. 1 from the main text to the data.

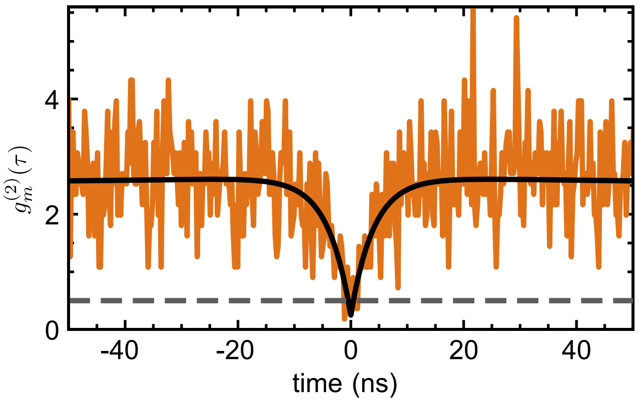


FIG. 1. A measured second order correlation function of the studied GeV center. The fit to Eq. 1 from the main text is shown with a solid line, while 0.5 is indicated with a dashed line for reference.

For the measurement in Fig. 1, we obtain $\tau_1 = 4.0 \pm 0.5$ ns, $\tau_2 = 1.19 \pm 0.01$ ms, $a = 2.2 \pm 0.4$, and

$\sigma^2 = 0.75 \pm 0.16$, resulting in $g_m^{(2)}(0) = 0.25 \pm 0.16$. Thus the deviation from the expected condition $g^2(0) = 0$ is fully explained by the presence of Poissonian background, proving that the observed GeV center is a single emitter.

## III. RATE ANALYSIS

We fit a series of power-dependent $g_m^{(2)}$ measurements using Eq. 1 from the main text to obtain information regarding the population dynamics of our system (Figs. 3a and b from the main text). Here, we look at correlations over a large range of time scales to observe a long-lived shelving state in the electronic level structure. The clear bunching of the $g_m^{(2)}$ function at high excitation powers implies that there are at least three states involved in the dynamics. In practice, we found that our data could be well described by an effective three-level model (Fig. 3c from the main text), where 1 and 2 are the ground and excited states respectively and 3 is an additional shelving state, which has been postulated to be a different GeV charge state [37]. A standard three-level model with $k_{12}$ as the only power-dependent rate does not fit the data; we therefore include ionization from the excited and shelving states with linear power dependence. Such a model has been used successfully in describing the rates of single SiV centers [34, 39]. The power-dependent intersystem rates are either proportional to power (yellow in Fig. 3c from the main text) or have linear and constant terms (red arrow) according to

$$k_{12} = c_{12} P \tag{1}$$
$$k_{32} = c_{32} P \tag{2}$$
$$k_{23} = c_{23} P + k_{23}^0, \tag{3}$$

where $k_{23}^0$ and $c_{ij}$ are constants. The rates $k_{21}$ and $k_{31}$ are assumed to be independent of excitation power (green arrows). The fitting parameters in Eq. 1 from the main text are related to these intersystem rates by

$$\tau_{1,2} = \frac{2}{\left(A \pm \sqrt{A^2 - 4B}\right)} \tag{4}$$
$$a = \frac{1 - \tau_2 \left(k_{31} + k_{32}\right)}{\left(k_{31} + k_{32}\right)\left(\tau_2 - \tau_1\right)}, \tag{5}$$

where

$$A = k_{12} + k_{21} + k_{23} + k_{31} + k_{32} \tag{6}$$
$$B = k_{23}k_{31} + k_{21}\left(k_{31} + k_{32}\right) + k_{12}\left(k_{23} + k_{31} + k_{32}\right). \tag{7}$$

Fits to the three-level model are shown with black lines in Figs. 3a and b from the main text, leading to the extracted rates of

$$c_{12} = 2.3 \pm 0.4 \text{ MHz/mW}$$
$$c_{23} = 0.29 \pm 0.04 \text{ MHz/mW}$$
$$c_{32} = 12.3 \pm 0.2 \text{ kHz/mW}$$
$$k_{23}^0 = 1.5 \pm 0.3 \text{ MHz}$$
$$k_{21} = 165 \pm 3 \text{ MHz}$$
$$k_{31} = 7.6 \pm 1.5 \text{ kHz}.$$

From these parameters, the steady-state populations of each level can be estimated as a function of excitation power (Fig. 3d in the main text), resulting in a dark state population of $96 \pm 18\%$ at infinite pump power.

## IV. WHITE LIGHT CAVITY TRANSMISSION

Geometric cavity parameters can be extracted by characterizing the broadband cavity transmission spectrum as a function of cavity length. We couple a white light laser (NKT Photonics) through the fiber

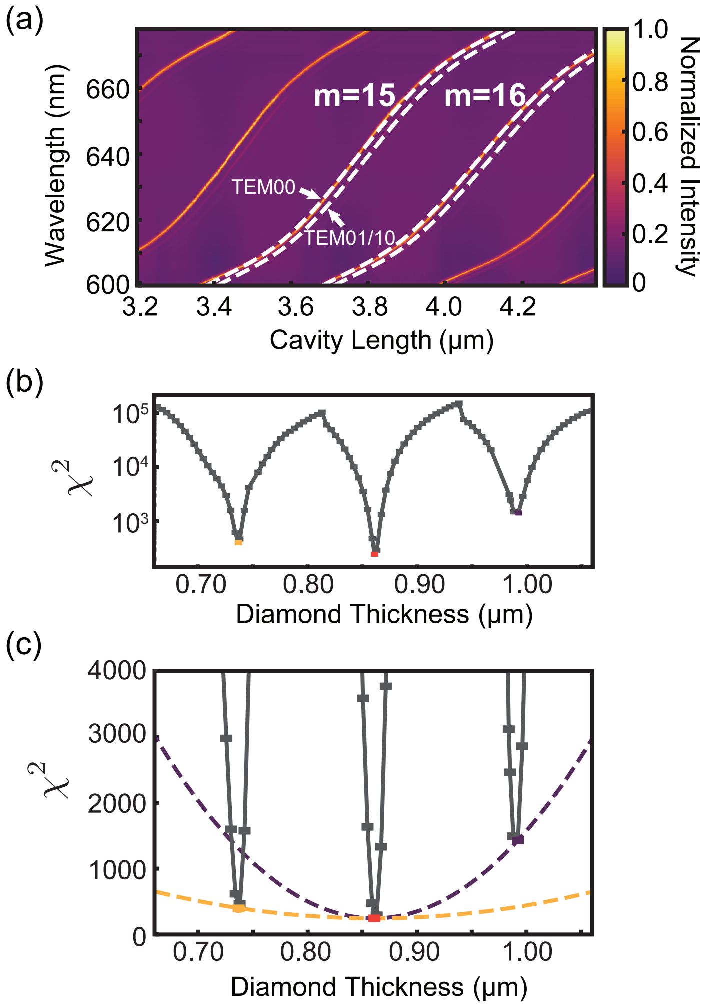


FIG. 2. Broadband cavity transmission as a function of length. The dashed lines correspond to numerical fits to the fundamental (TEM00) and first-order transverse (TEM01/10) modes for the $m = 15$ and 16 longitudinal modes. b) A one-dimensional cut of the $\chi^2$ landscape for fitting $t_d$ (shown in log-scale to illustrate the approximate periodicity). Local minima are shown in yellow, orange, and purple. c) The same $\chi^2$ local minima plotted with linear-scale. To calculate the error on $t_d$, we fit a parabola to the overall global minimum (orange) and each of the adjacent minima (purple and yellow). The asymmetric error bounds on $t_d = 862^{+1}_{-4}$ nm correspond to the $\chi^2_{min} + 1$ points on these parabolas.

mirror and collect transmission through the flat mirror, revealing the mode structure (Fig. 2a). We fit the fundamental and first order transverse modes of two adjacent longitudinal modes to a transfer matrix model including Gouy phase (dashed lines in Fig. 2a [31]). From this fit, we extract a membrane thickness $t_d = 862^{+1}_{-4}$ nm, radius of curvature $R = 43.1 \pm 0.6$ μm, as well as the mode numbers $m$ and cavity lengths $L$ labeled on the plot. The $m = 15$ resonance was the lowest longitudinal mode number achievable before the fiber mirror made physical contact with the membrane.

We provide more details on the fitting procedure of $t_d$ by showcasing a one-dimensional cut of the $\chi^2$ landscape (Figs. 2b-c). We find that $\chi^2$ is approximately periodic in $t_d$ (visible in Fig. 2b), where each local minimum (shown in yellow, orange, and purple) has a corresponding set of best fit parameters. To find the global minimum ($\chi^2_{min}$), we execute a least-squares fit over a grid of possible minima and retain the lowest value (shown in orange). To calculate the error on this value, we fit a parabola to the overall global minimum and each of the adjacent minima (purple and yellow traces in Fig. 2c). The asymmetric error bounds on $t_d$ then correspond to the $\chi^2_{min} + 1$ points on these parabolas, which is consistent with the variation in $t_d$ obtained by fitting a series of white light data sets measured in the same region of another membrane

sample. We note that the extracted error is an order of magnitude larger than what was obtained through least-squares fitting. Finally, using the extracted value of $t_d$ as an initial guess, we perform a Nelder-Mead fitting algorithm in the vicinity of the minimum to determine the final values of $t_d$ and $R$.

In addition, we use the cavity transmission spectrum to estimate the cavity decay rate. We first measure the cavity linewidth to be $\Delta L = 27 \pm 4$ pm, corresponding to a finesse of $\mathcal{F}_L = \lambda/(2\,\Delta L) = 11,200 \pm 1{,}700$. The magnitude of the slope of the $m = 15$ resonance at 603 nm is $40 \pm 2$ THz/μm, corresponding to a decay rate of $\kappa/(2\pi) = 1.08 \pm 0.17$ GHz.

## V. ASYMMETRIC ERROR PROPAGATION

Several results in this manuscript are reported with asymmetric errors stemming from the dipole emission fiber coupling efficiency (see Sec. VI A for details). We illustrate our procedure for asymmetric error propagation using a general calculation of the quantity $Y^{+y_1}_{-y_2}$ (where $y_1$ and $y_2$ represent the positive and negative error bars on $Y$), which is a function of the parameter $X^{+x_1}_{-x_2}$. We calculate each $y_i$ using the direction of $x_i$ that corresponds to the sign of $\frac{\partial Y}{\partial X}$. Explicitly, $y_1$ is calculated using $x_1$ if the derivative is positive and $x_2$ if the derivative is negative, while $y_2$ is calculated in the opposite manner.

## VI. COLLECTION EFFICIENCY CALCULATIONS

Comparison of the saturating fluorescence counts in the confocal and cavity systems necessitates careful characterization of the measurement collection efficiencies. To extract the GeV center free-space emission from the confocal measurements, we first simulate the possible dipole emission patterns for our system including the membrane and mirror coating geometry (see Sec. VI A for details). This allows us to estimate that $0.23 \pm 0.03$ of emission escapes the diamond membrane (is not trapped in the form of guided modes); of this, $0.38 \pm 0.03$ is directed toward the objective (rather than into the flat mirror). Finally, we calculate a fiber-coupling efficiency of $0.55^{+0.11}_{-0.22}$ for an optical dipole along the $\langle 111 \rangle$ crystallographic axis. We must further correct for spectral filtering, which can be estimated by integrating the GeV center spectrum (see Fig. 6a, Sec. VIII A) between 600-605 nm ($\approx 496 - 500$ THz), resulting in a factor of $0.272 \pm 0.004$. Additional collection efficiencies exclusive to the confocal detection path are detailed in Tab. I.

| Optical Element | Collection Efficiency |
|---|---|
| emission toward objective | 0.38 ± 0.03 |
| membrane escape efficiency | 0.23 ± 0.03 |
| dipole emission fiber coupling | $0.55^{+0.11}_{-0.22}$ |
| spectral filtering | 0.272 ± 0.004 |
| objective transmission (603 nm) | 0.80 ± 0.01 |
| 2 dielectric mirrors | 0.98 ± 0.01 |
| total $\eta_{free,ex}$ | $0.010^{+0.003}_{-0.004}$ |

TABLE I. Confocal optical elements.

Similarly, all of the collection efficiencies exclusive to the cavity setup are listed in Tab. II. The flat mirror escape efficiency provides the normalized transmission through the flat mirror including all cavity losses (cavity transmission, scattering, and absorption, as well as reflection from the back mirror interface). Using our transfer matrix model, we estimate this quantity to be $0.265 \pm 0.008$ at 603 nm for the $m = 15$ mode, where the error is estimated using the values at 600 and 605 nm and the error on $t_d$. The cavity is designed to be critically coupled (matching transmission through fiber and flat mirrors in the absence of scattering and absorption). We assume that all photons emitted through the flat mirror are collected by the objective due to the comparatively low NA of the cavity mode ($\approx 0.1$). We image the collimated cavity mode yielding a beam radius of $690 \pm 70$ μm, which is used to calculate a fiber coupling efficiency of $0.89 \pm 0.09$ (this is an upper bound which assumes perfect lateral alignment and neglects aberrations). We only consider emission

coupled to a fundamental cavity mode, and correct for coupling to higher order transverse modes with a factor of $1.25 \pm 0.08$ (see Sec. VI B).

| Optical Element | Collection Efficiency |
|---|---|
| flat mirror escape efficiency | 0.265 ± 0.008 |
| objective transmission (603 nm) | 0.91 ± 0.01 |
| 4 dielectric mirrors | 0.96 ± 0.02 |
| dichroic transmission | 0.93 ± 0.01 |
| collection fiber coupling | 0.89 ± 0.09 |
| transverse mode contribution | 1.25 ± 0.08 |
| total $\eta_{cav,ex}$ | 0.24 ± 0.03 |

TABLE II. Cavity optical elements.

Finally, there are a number of optical components that are common to both the cavity and confocal setups detailed in Tab. III.

| Optical Element | Collection Efficiency |
|---|---|
| fiber coupling lens | 1.00 ± 0.01 |
| tunable long pass filter | 0.92 ± 0.02 |
| tunable short pass filter | 0.92 ± 0.02 |
| 532 nm notch filter | 0.97 ± 0.02 |
| transmission at fiber facets | 0.94 ± 0.03 |
| APD telescope lenses | 0.98 ± 0.02 |
| APD efficiency (600 nm) | 0.45 ± 0.02 |
| total $\eta_{comm}$ | 0.34 ± 0.02 |

TABLE III. Common optical elements.

The measured free-space and cavity counts should therefore be corrected by $\eta_{free} = \eta_{free,ex}\,\eta_{comm} = (3.5^{+0.9}_{-1.5}) \times 10^{-3}$ and $\eta_{cav} = \eta_{cav,ex}\eta_{comm} = 0.082 \pm 0.012$ respectively, where we attribute units of counts/photon to these efficiencies since they convert detector counts to emitted photons.

### A. Dipole Emission Calculation

We calculate the directional emission pattern of the GeV center to estimate the collection efficiency of our confocal setup. To that end, we model the spontaneous emission from a GeV as that of a classical dipole (this assumption is valid as the spatial extent of the GeV is much smaller than the emission wavelength and the transition orbital is not affected by the dielectric mirror [55]). For these calculations, we consider a dipole positioned $h = 125 \pm 20$ nm above the flat mirror in a diamond layer with thickness $t_d = 862$ nm (see Fig. 3). The mirror coating is modeled with 50 alternating layers of $SiO_2$ and $Ta_2O_5$ with the design layer thicknesses $t_i$, deposited on a fused silica substrate. We find that the collection efficiency is limited by three factors: light confinement in the membrane due to total internal reflection, the ratio of light emitted toward the objective verses into the flat mirror, and the overlap of the dipole emission field with the mode of our collection fiber.

The first two considerations are evaluated using a model developed by Lukosz and Kunz [55] and further extended by Neyts [56]. We find that the micron-scale thickness and high refractive index of diamond makes it an efficient waveguide. Consequently, much of the GeV emission is trapped in guided diamond modes depending on the angle $\alpha$. The optical dipole orientation of the GeV center has not been experimentally

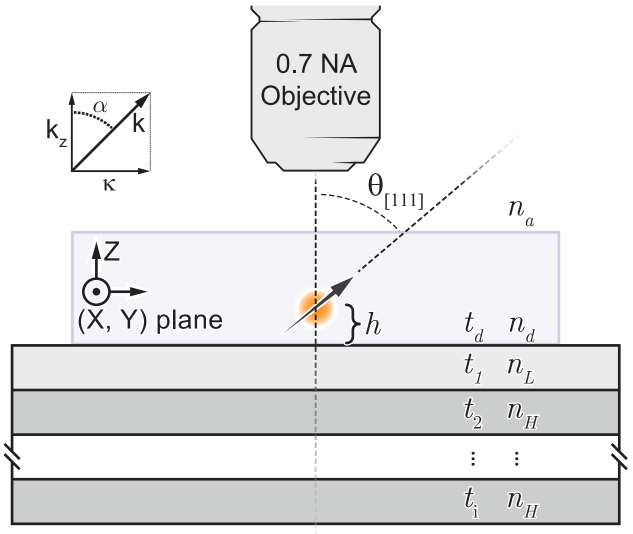


FIG. 3. An illustration of the dipole simulation parameters.

determined, but by symmetry we assume that it is either a single dipole along the ⟨111⟩ directions, or two perpendicular dipoles in the (111) plane. Considering both of these cases, we find a membrane escape efficiency of $0.23 \pm 0.03$. Furthermore, we find that only a fraction of $0.38 \pm 0.03$ of the far-field emission is directed toward the objective. This is surprising since the Bragg stack is designed to be highly reflective at this wavelength, but was optimized for plane waves as opposed to the more-complicated dipole emission we consider here. Moving forward, it may be possible to numerically optimize the layer thicknesses to take into account the full dipole radiation pattern.

Finally, we calculate the overlap of the dipole emission (collected by the 0.7 NA objective) with a single mode fiber using a transfer-matrix method [57] facilitated by the Lorentz reciprocity theorem as described in the Appendix of [58]. Here, we consider a dipole along the ⟨111⟩-axis, neglect aberrations from lenses, and assume the fiber is placed in the focal plane of the last lens, resulting in an efficiency of $0.47^{+0.11}_{-0.22}$. The relatively large error comes from uncertainties on the fiber mode field diameter ($4.0 \pm 0.5$ μm) and ion implantation depth ($125 \pm 20$ nm). Defocusing the fiber coupling lens expands the collected beam to better match the fiber diameter, which systematically improves this value by a factor of $(7.15^{+0.01}_{-1.15}) \times 10^{-2}$, resulting in a final collection efficiency of $0.55^{+0.11}_{-0.22}$.

### B. Higher Order Modes

Our analysis assumes that we only collect emission coupled to a fundamental cavity mode as the single mode fiber in our collection path should spatially filter out other transverse modes. In practice, we do collect some emission coupled to higher order modes (see Fig. 4), comprising $20 \pm 5\%$ of the total emission in this particular scan. We attribute this to lateral misalignment of the cavity mode on the collection fiber, which may vary slightly over time due to experimental drift and realignment. The count rate from the fundamental cavity mode is therefore $I_{fund,meas} = I_{cav,meas}/\eta_{hotm}$ with the correction factor $\eta_{hotm} = 1.25 \pm 0.08$ for higher order transverse modes.

## VII. POWER SPECTRAL DENSITY CALCULATIONS

Cavity funneling is evidenced by an increase in the spectral density of GeV emission in the cavity compared to the confocal configuration. We quantify this effect through comparison of the peak spectral density of

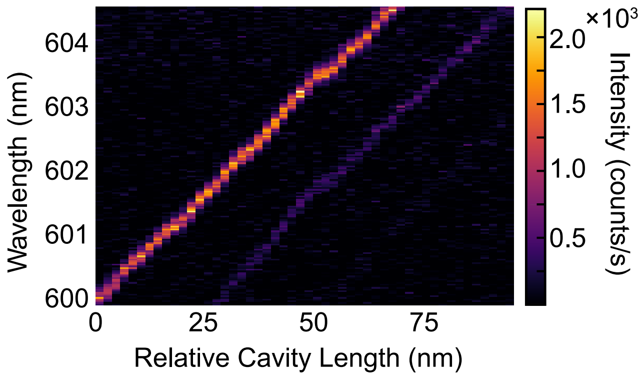


FIG. 4. GeV center fluorescence as a function of cavity length. A weak higher order mode is visible at shorter wavelengths compared to the bright fundamental mode for a fixed cavity length.

emission given by

$$PSD = \max_{\nu \in [\nu_1, \nu_2]} \{SD(\nu)\}, \tag{8}$$

where $SD(\nu)$ is the spectral density as a function of frequency $\nu$ over the spectral filtering range $[\nu_1, \nu_2]$. We consider emission with a Lorentzian lineshape given by

$$SD(\nu) = \frac{I^\infty}{\pi} \frac{(b/2)}{(b/2)^2 + (\nu - \nu_0)^2}, \tag{9}$$

where $b$ is the FWHM linewidth, $\nu_0$ is the center frequency (which is assumed to fall within the filtered frequency range), and $I^\infty$ is the total (corrected) integrated counts, such that $\int_{-\infty}^{\infty} SD(\nu)\, d\nu = I^\infty$. The corrected ($I^\infty$) and measured ($I^\infty_{meas}$) counts are related by $I^\infty = I^\infty_{meas}/\eta\zeta$, where $\eta$ is the photon collection efficiency and $\zeta$ parameterizes the spectral filtering window according to $\int_{\nu_1}^{\nu_2} SD(\nu)\, d\nu = \zeta I^\infty$. The peak spectral density can then be calculated as a function of the measured saturating fluorescence counts as

$$PSD = \frac{2I^\infty}{\pi b} = \frac{2}{\pi b} \frac{I^\infty_m}{\eta\zeta}. \tag{10}$$

For the cavity setup, we collect emission within the full cavity linewidth $b = \kappa/(2\pi)$ ($\xi = 1$). Using $\eta = \eta_{cav}$ and $I^\infty_{cav,meas} = 380 \pm 50$ counts/s we calculate $PSD_{cav} = 2{,}800 \pm 700$ counts/(s GHz).

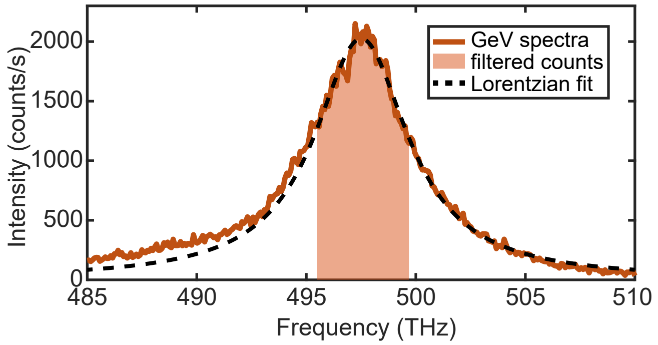


FIG. 5. GeV spectrum in the confocal setup. A Lorentzian fit to the ZPL with $\gamma^*/(2\pi)$ =5.22 THz is shown in the black dashed line, while the shaded region represents our filtering window.

In the confocal configuration, we collect emission between $\approx 600 - 605$ nm, corresponding to $\zeta = 0.426 \pm 0.005$ of the total ZPL emission (the shaded region in Fig. 5). The collection efficiency is $\eta = \eta_{free}/\eta_{filt}$, where $\eta_{filt} = 0.272 \pm 0.004$ is the filtering correction applied to extract the total freespace emission in the main text. The relevant linewidth is the pure dephasing rate $b = \gamma^*/(2\pi)$ and the measured saturating fluorescence count rate is $I^\infty_{con,meas} = 4{,}000 \pm 200$ counts/s, resulting in $PSD_{con} = 90^{+40}_{-20}$ counts/(s GHz).

## VIII. CAVITY FUNNELING THEORY

We calculate the efficiency of emission into the cavity mode $\beta$ by modeling the GeV center as an emitter with $n$ optical transitions [33]

$$\beta = \frac{\sum_{j=0}^{n-1} R_j}{\gamma + \sum_{j=0}^{n-1} R_j}, \tag{11}$$

where $R_j$ is the emitter-cavity coupling rate of the $j$th transition. In the bad emitter limit ($\gamma_j^* \gg \gamma + \kappa$), this is given by

$$R_j = \frac{4g_j^2}{\gamma_j^*} \frac{1}{1 + \left(\frac{2\delta_j}{\gamma_j^*}\right)^2}, \tag{12}$$

where $g_j$ is the coupling rate of the $j$th transition to the cavity (which is related to the overall coupling rate $g$ by the branching ratio $\xi_j$ by $g_j = \sqrt{\xi_j} g$), $\delta_j$ is the transition-cavity detuning, and $\gamma_j^*$ is the homogeneous dephasing rate [33]. If the cavity is resonantly coupled to the ZPL transition ($i = 0$), emission from the phonon sideband (PSB) transitions into the cavity mode can be neglected if

$$\frac{\xi_0}{\gamma_0^*} \gg \sum_{j \neq 0} \frac{\xi_j}{\gamma_j^*} \frac{1}{1 + \left(\frac{2\delta_j}{\gamma_j^*}\right)^2}. \tag{13}$$

For the case of the GeV center, we find that the PSB transitions contribute negligibly to the cavity emission when on resonance with the ZPL (analysis in Sec. VIII A) and the total efficiency can then be approximated as $\beta = R_0/(\gamma + R_0)$. The total cavity-coupling rate is given by

$$g = \sqrt{\frac{3\,c\,\lambda^2\,\gamma}{8\pi\,n_d^3\,V}} \frac{\left|\vec{f}(z_0)\cdot\vec{\mu}\,\right|}{|\vec{\mu}|}, \tag{14}$$

where $\vec{\mu}$ is the optical dipole moment of the emitter, $\vec{f}(z_0)$ is a complex vector describing the electric field polarization and normalized amplitude at the position of the emitter ($z_0$), $n_d$ is the refractive index of diamond, and $V$ is the cavity mode volume, given approximately by

$$V = \frac{\pi\omega_0^2}{2} \frac{\int n^2(z)|E(z)|^2 dz}{n_d^2 |E(z_0)|^2}, \tag{15}$$

where $\omega_0$ is the cavity waist radius and $E(z)$ is the cavity electric field at position $z$ along the cavity axis.

With these equations, we can calculate $\beta$ by simulating the electric field distribution of the cavity mode using one-dimensional transfer matrix theory [31], where we use the measured dephasing rate $\gamma^* = 2\pi \times 5.22$ THz (see below), ZPL wavelength $\lambda = 603$ nm, and a Debye-Waller factor of $\xi = 0.6$ [43]. We assume that the optical dipole is along the $\langle 111 \rangle$-axis, as is approximately the case for the SiV center [19]. Absorption losses in the mirrors are included through the addition of complex components in the dielectric layer refractive indices, lowering the bare cavity finesse to the observed value $\mathcal{F} \approx 21,000$ at 652.6 nm. In addition, scattering losses are introduced by adding $\sigma = 0.16$ nm-rms of surface roughness to the diamond interfaces [31, 59, 60], reducing the membrane-in-cavity finesse to the measured value of $\mathcal{F} \approx 11,000$ at 603 nm. We assume that the flat mirror surface does not exactly follow the membrane morphology due to roughness; consequently, we include an infinitely thin air layer between the diamond and flat for our calculation of scattering losses. Finally, we use a fiber mirror radius of $R = 43.1$ µm and diamond thickness $t_d = 862$ nm (see section IV for details), and include lensing effects on the cavity mode from the planar diamond-air interface in calculating the cavity waist diameter [61].

### A. Spectra Fitting

In the previous section, we neglected contributions from the PSB transitions. Here, we show the validity of this approximation by estimating the emission into the cavity mode from PSB transitions when on resonance

with the ZPL. To do this, we analyze the spectrum of the emitter from 585-630 nm ($\approx 476 - 513$ THz), over which we assume the response of our optics and detector are constant. To account for background from the diamond, we took a spectrum on (Fig. 6a, orange trace) and off (yellow trace) the studied GeV center. The high signal to noise ratio achieved in our confocal scans between 600-605 nm ensured that this background was not coming from an emitter, and indeed it agrees well with published data on the second-order Raman transition in diamond for 532 nm excitation [21, 62]. We correct the raw GeV spectrum using this background by normalizing to the area under the first order Raman transition in each scan before subtraction, resulting in the purple trace in Fig. 6a.

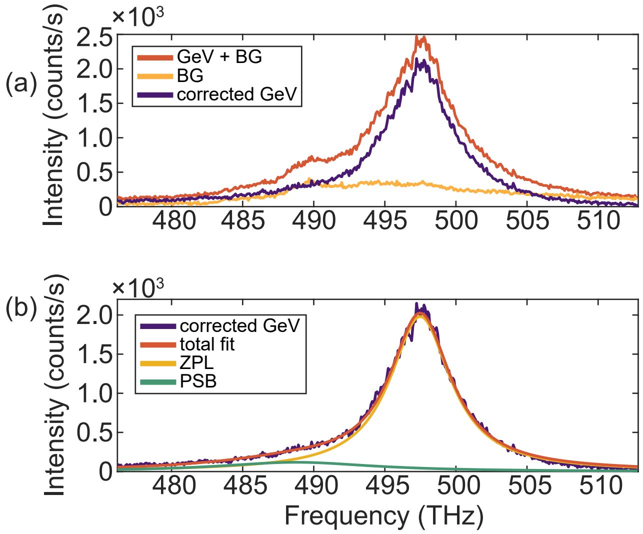


FIG. 6. a) A raw GeV spectrum (orange), background diamond spectrum (yellow), and the corrected GeV spectrum (purple). b) A two-Lorentzian fit (orange) to the corrected GeV spectrum (purple), with the individual contributions of the ZPL (yellow) and PSB (green) plotted.

The corrected spectrum was fit to the sum of two Lorentzians (of the form $I(\nu) = A\frac{(\gamma^*/4\pi)}{(\gamma^*/4\pi)^2+(\nu-\nu_0)^2}$) with zero constant offset (orange trace, Fig. 6b), representing the ZPL transition (yellow), and a broad PSB transition (green), with fit parameters listed in Tab. IV.

| Parameter | ZPL | PSB |
|---|---|---|
| A (counts·THz) | 5170±60 | 790±90 |
| $\gamma^*/(2\pi)$ (THz) | $5.22 \pm 0.05$ | 13.4±1.4 |
| $\nu_0$ (THz) | 497.491±0.012 | $488.8 \pm 0.5$ |

TABLE IV. Spectrum fit parameters.

Comparing the integrated counts for each of these transitions results in 87% of the photons occurring in the ZPL. The Huang-Rhys factor for the GeV center was reported to be approximately 0.5 [43], resulting in a ZPL branching ratio of 60%. We therefore conclude that the fitted PSB transition comprises 9% of the total emission, and the other 31% of the PSB emission must occur at longer wavelengths. Considering only the fitted transitions, we find that it is valid to neglect contributions from the PSB when the cavity is on resonance with the ZPL, since

$$\left(\frac{\epsilon_{ZPL}}{\gamma^*_{ZPL}}\right) \Bigg/ \left(\frac{\epsilon_{PSB}}{\gamma^*_{PSB}} \frac{1}{1+\left(\frac{2\delta_{PSB}}{\gamma^*_{PSB}}\right)^2}\right) \approx 50, \tag{16}$$

where $\delta_{PSB} = 2\pi \times (\nu_{0,ZPL} - \nu_{0,PSB})$. We can therefore also neglect contributions from other PSB transitions which are necessarily further detuned, and assume that only photons from the ZPL are emitted into the cavity mode.

---

* R. H. J. and E. J. contributed equally to this work.; corresponding authors: rasjen@fysik.dtu.dk and erika.janitz@mail.mcgill.ca
[19] L. J. Rogers, K. D. Jahnke, M. W. Doherty, A. Dietrich, L. P. McGuinness, C. Müller, T. Teraji, H. Sumiya, J. Isoya, N. B. Manson, *et al.*, Electronic structure of the negatively charged silicon-vacancy center in diamond, Physical Review B **89**, 235101 (2014).
[21] T. Iwasaki, F. Ishibashi, Y. Miyamoto, Y. Doi, S. Kobayashi, T. Miyazaki, K. Tahara, K. D. Jahnke, L. J. Rogers, B. Naydenov, *et al.*, Germanium-Vacancy Single Color Centers in Diamond, Scientific Reports **5**, 12882 (2015).
[31] E. Janitz, M. Ruf, M. Dimock, A. Bourassa, J. Sankey, and L. Childress, Fabry-Perot microcavity for diamond-based photonics, Physical Review A **92**, 043844 (2015).
[33] R. Albrecht, A. Bommer, C. Deutsch, J. Reichel, and C. Becher, Coupling of a Single Nitrogen-Vacancy Center in Diamond to a Fiber-Based Microcavity, Physical Review Letters **110** (2013).
[34] J. Benedikter, H. Kaupp, T. Hümmer, Y. Liang, A. Bommer, C. Becher, A. Krueger, J. M. Smith, T. W. Hänsch, and D. Hunger, Cavity-Enhanced Single-Photon Source Based on the Silicon-Vacancy Center in Diamond, Physical Review Applied **7**, 024031 (2017).
[37] D. Chen, Z. Mu, Y. Zhou, J. E. Fröch, A. Rasmit, C. Diederichs, N. Zheludev, I. Aharonovich, and W.-b. Gao, Optical Gating of Resonance Fluorescence from a Single Germanium Vacancy Color Center in Diamond, Physical Revivew Letters **123**, 033602 (2019).
[39] E. Neu, M. Agio, and C. Becher, Photophysics of single silicon vacancy centers in diamond: implications for single photon emission, Optics Express **20**, 19956 (2012).
[43] Y. N. Palyanov, I. N. Kupriyanov, Y. M. Borzdov, and N. V. Surovtsev, Germanium: a new catalyst for diamond synthesis and a new optically active impurity in diamond, Scientific Reports **5**, 14789 (2015).
[50] B. J. M. Hausmann, B. Shields, Q. Quan, P. Maletinsky, M. McCutcheon, J. T. Choy, T. M. Babinec, A. Kubanek, A. Yacoby, M. D. Lukin, *et al.*, Integrated Diamond Networks for Quantum Nanophotonics, Nano Letters **12**, 1578 (2012).
[51] P. Latawiec, V. Venkataraman, M. J. Burek, B. J. Hausmann, I. Bulu, and M. Lončar, On-chip diamond Raman laser, Optica **2**, 924 (2015).
[52] P. Appel, E. Neu, M. Ganzhorn, A. Barfuss, M. Batzer, M. Gratz, A. Tschöpe, and P. Maletinsky, Fabrication of all diamond scanning probes for nanoscale magnetometry, Review of Scientific Instruments **87**, 063703 (2016).
[53] J. F. Ziegler, M. D. Ziegler, and J. P. Biersack, SRIM –The stopping and range of ions in matter (2010), Nuclear Instruments and Methods in Physics Research Section B: Beam Interactions with Materials and Atoms **268**, 1818 (2010).
[54] Y. Chu, N. de Leon, B. Shields, B. Hausmann, R. Evans, E. Togan, M. J. Burek, M. Markham, A. Stacey, A. Zibrov, *et al.*, Coherent Optical Transitions in Implanted Nitrogen Vacancy Centers, Nano Letters **14**, 1982 (2014).
[55] W. Lukosz and R. E. Kunz, Light emission by magnetic and electric dipoles close to a plane interface. I. Total radiated power, Journal of the Optical Society of America **67**, 1607 (1977).
[56] K. A. Neyts, Simulation of light emission from thin-film microcavities, Journal of the Optical Society of America A **15**, 962 (1998).
[57] L. Polereckỳ, J. Hamrle, and B. D. MacCraith, Theory of the radiation of dipoles placed within a multilayer system, Applied Optics **39**, 3968 (2000).
[58] C. Reed, J. Giergiel, J. Hemminger, and S. Ushioda, Dipole radiation in a multilayer geometry, Physical Review B **36**, 4990 (1987).
[59] C. C. Katsidis and D. I. Siapkas, General transfer-matrix method for optical multilayer systems with coherent, partially coherent, and incoherent interference, Applied Optics **41**, 3978 (2002).
[60] O. Arnon, Loss mechanisms in dielectric optical interference devices, Applied Optics **16**, 2147 (1977).
[61] S. B. van Dam, M. Ruf, and R. Hanson, Optimal design of diamond-air microcavities for quantum networks using an analytical approach, New Journal of Physics **20**, 115004 (2018).
[62] S. A. Solin and A. K. Ramdas, Raman Spectrum of Diamond, Physical Review B **1**, 1687 (1970).
